# Supplementary material for: EM's Convergence in Gaussian Latent Tree Models
Source: arXiv:2211.11904 source file (2022-11-23)
Supplement: Supplementary file 1 [file to-appendix.tex]

\begin{proof}[Proof of Claim~\ref{cla:lambda}]
\yuval{move down, and fill the details}
It holds that
\[
\E[x_i \mid y] = \frac{\sigma_{x_i}\rho_{i}}{\sigma_y}y\enspace.
\]
From this we can derive that
\[
\Cov(x_i,x_j)
= \E[x_i x_j]
= \E[\E[x_i x_j \mid y]]
= \E[\E[x_i \mid y]\E[x_j \mid y]] 
= \E[\frac{\sigma_{x_i} \sigma_{x_j}\rho_i\rho_j}{\sigma_y^2}y^2]
= \sigma_{x_i} \sigma_{x_j}\rho_i\rho_j.
\]
This completely determines the covariance matrix as a function of $\sigma_y^2$ and the parameters $\sigma_{x_i}^2,\rho_i$ for $i =1,\dots,n$. Lastly, we note that conditionally on $x_1,\dots,x_n$, one has

Further, $\Var[y\mid x_1 \cdots x_n]$ is independent of the values of $x_1,\dots,x_n$.
\end{proof}
